# Supplementary material for: Generalization Guarantees for Neural Networks via Harnessing the Low-rank Structure of the Jacobian
Source: arXiv:1906.05392 source file (2019-07-04)
Supplement: Supplementary file 1 [file numerics_appendix.tex]

% !TEX root = shorter_arxiv.tex
%\section{Futher numerical experiments}\label{numeric apx}

%Table \ref{exp:table_nolc_apx} summarizes important metrics we tracked in our first experiment with no label corruption. Adaptation of the Jacobian after training is demonstrated by the significant increase in both label and initial residual energy falling onto the information subspace with a consequent decrease in energy on the nuisance subspace while $\twonorm{\mtx{J}_{\calF}^{\dagger}\y}$ remains relatively small resulting in better generalization.  
%
%We still observed Jacobian adaptation in the label corruption experiment, however to a smaller degree (Table \ref{exp:table_lc50_apx}). Due to corruption, labels are less correlated with the information subspace of the Jacobian and energy on the nuisance subspace increases resulting in worse generalization.
%
%
%		\centering
%		\resizebox{\textwidth}{!}
%		{
%		\begin{tabular}{|l||c|c|c||c|c|r|}
%			\hline
%			&$\frac{\twonorm{\Pi_{\calF}( \y)}}{\twonorm{\y}}$ & %y_F
%			$\frac{\twonorm{\Pi_{\calS}( \y)}}{\twonorm{\y}}$ & %y_S
%			$\frac{\twonorm{\mtx{J}_{\calF}^{\dagger}\y}}{\twonorm{\y}}$ & % pinv y
%			$\frac{\twonorm{\Pi_{\calF}( \vct{r}_0)}}{\twonorm{\vct{r}_0}}$  & %r_F
%			$\frac{\twonorm{\Pi_{\calS}( \vct{r}_0)}}{\twonorm{\vct{r}_0}}$ & %r_S
%			$\frac{\twonorm{\mtx{J}_{\calF}^{\dagger}\vct{r}_0}}{\twonorm{\vct{r}_0}}$ \\%pinv r
%			\hlineB{2.5}
%			\textbf{$\mtx{J}_{init}$} & 0.72 &  0.69 & $5.4\cdot 10^{-3}$&  0.89  & 0.46& $4.1\cdot 10^{-3}$\\
%			\hline
%			\textbf{$\mtx{J}_{final}$} & 0.99 &  0.16 &  $3.2\cdot 10^{-3}$&  0.98  & 0.22&$3.4\cdot 10^{-3}$\\
%		%	\textbf{Initial $\mtx{J}$, test }&  0.73366 &  0.67951 &  0.010328 & 0.88827&  0.45932 & 0.0077364\\
%		%	\textbf{Final $\mtx{J}$, test }&  0.8974 &  0.44123 &  0.0027082 & 0.89772&  0.44057 & 0.0029383\\
%			\hline
%		\end{tabular}
%	}
%	\captionof{table}{Depiction of the alignment of the initial label/residual with the information/nuisance space using uncorrupted data and a Multi-class ResNet20 model}\label{exp:table_nolc_apx}
%			\resizebox{\textwidth}{!}
%	{
%		\begin{tabular}{|l||c|c|c||c|c|r|}% <-- Alignments: 1st column left, 2nd middle and 3rd right, with vertical lines in between
%			\hline
%			&$\frac{\twonorm{\Pi_{\calF}( \y)}}{\twonorm{\y}}$ & %y_F
%			$\frac{\twonorm{\Pi_{\calS}( \y)}}{\twonorm{\y}}$ & %y_S
%			$\frac{\twonorm{\mtx{J}_{\calF}^{\dagger}\y}}{\twonorm{\y}}$ & % pinv y
%			$\frac{\twonorm{\Pi_{\calF}( \vct{r}_0)}}{\twonorm{\vct{r}_0}}$  & %r_F
%			$\frac{\twonorm{\Pi_{\calS}( \vct{r}_0)}}{\twonorm{\vct{r}_0}}$ & %r_S
%			$\frac{\twonorm{\mtx{J}_{\calF}^{\dagger}\vct{r}_0}}{\twonorm{\vct{r}_0}}$ \\%pinv r
%			\hlineB{2.5}
%			\textbf{$\mtx{J}_{init}$} & 0.59&  0.81 & $1.7\cdot 10^{-3}$&  0.64  & 0.77& $2.0\cdot 10^{-3}$\\
%			\hline
%			\textbf{$\mtx{J}_{final}$} & 0.75 &  0.66 & $1.8\cdot 10^{-3}$ &  0.76  & 0.6& $1.2\cdot 10^{-3}$\\
%			%	\textbf{Initial $\mtx{J}$, test }&  0.7236 &  0.69021 &  0.012765 & 0.7594&  0.65062 & 0.01235\\
%			%	\textbf{Final $\mtx{J}$, test }&  0.75362 &  0.65731 &  0.0033476 & 0.77225&  0.63532 & 0.0021479\\
%			\hline
%		\end{tabular}
%	}
%	\captionof{table}{Depiction of the alignment of the initial label/residual with the information/nuisance space using 50\% label corrupted data and a Multi-class ResNet20 model}\label{exp:table_lc50_apx}
